# Supplementary material for: React-OT: Optimal Transport for Generating Transition State in Chemical Reactions
Source: arXiv:2404.13430 source file (2024-10-15)
Supplement: Supplementary file 1 [file SI.tex]

\appendix

% \title{\textit{Supplementary Information} for "Accurate transition state generation with an object-aware equivariant elementary reaction diffusion model"}

% \maketitle

\renewcommand{\thetable}{S\arabic{table}}  
\renewcommand{\thefigure}{S\arabic{figure}}
\setcounter{figure}{0}
\setcounter{table}{0}

\makeatletter
\renewcommand{\fnum@figure}{\textbf{Figure \thefigure}. }
\renewcommand{\fnum@table}{\textbf{Table \thetable. }}

\section*{Abbreviation}
The following is the list of abbreviation utilized in the main paper.
\begin{enumerate}
    \item OA-ReactDiff: \underline{O}bject-\underline{a}ware SE(3) GNN for generating sets of 3D molecules in elementary \underline{react}ions under the \underline{diff}usion model
    \item RMSD: Root mean square deviation.
    \item SE(3): Special Euclidean group in 3D space.
    \item TS: Transition state.
    \item MAE: Mean absolute error.

\end{enumerate}

% Physical symmetries and constraints in an elementary reaction
\section{Physical symmetries and constraints in an elementary reaction.}
\label{SI:required_symmetries}
An elementary reaction that consists of $n$ fragments as reactant and $m$ fragments as product can be described as $\{\mathrm{R}^{(1)}, ..., \mathrm{R}^{(n)}, \mathrm{TS}, \mathrm{P^{(1)}}, ...,  \mathrm{P^{(m)}}\}$. This reaction requires the following symmetries:
\begin{enumerate}
    \item \textit{Permutation symmetry among atoms in a fragment}. For any fragment in $\mathrm{R}^{(i)}, \mathrm{TS}, \mathrm{P^{(j)}}$, change of atom ordering preserves the reaction.
    \item \textit{Permutation symmetry among fragments in reactant and product}. The change of ordering in $\{\mathrm{R}^{(1)}, ..., \mathrm{R}^{(n)} \}$ and $\{\mathrm{P}^{(1)}, ..., \mathrm{P}^{(m)} \}$ preserve the reaction.
    \item \textit{Rotation and translation symmetry for each fragment}. Rotation and translation operations on any fragment (i.e., $\mathrm{R}^{(i)}, \mathrm{TS}, \mathrm{P^{(j)}}$) preserve the reaction.
\end{enumerate}

\section{Reaction network exploration with React-OT.}
\label{SI:reaction_network}
To demonstrate the practical application of React-OT in reaction network exploration, the reaction network of $\gamma$-ketohydroperoxide (KHP), a well-studied system commonly used as a benchmark in recent studies.\cite{grambow2018KHP,naz2020unimolecular,QiyuanNCS2021,zhao2022YARP2} Building on reactions generated via graph-based enumeration,\cite{QiyuanNCS2021} we utilized React-OT to determine transition states, which are then used to evaluate activation energies at $\omega$B97X/6-31G* level of theory. Based on predicted activation energies, a two-step reaction network was constructed and compared with the network generated using a DFT-based approach. Following a simple rule for reaction network growth, each node expansion allows the generation of up to five branches, prioritizing the reactions with the lowest energy barriers. The resulting networks generated by React-OT and traditional DFT approach have the identical nodes. This case study illustrates how React-OT can be applied to speed up the reaction network exploration.

\begin{figure*}[t!]
    % \centering
    \includegraphics[width=1.0\textwidth]{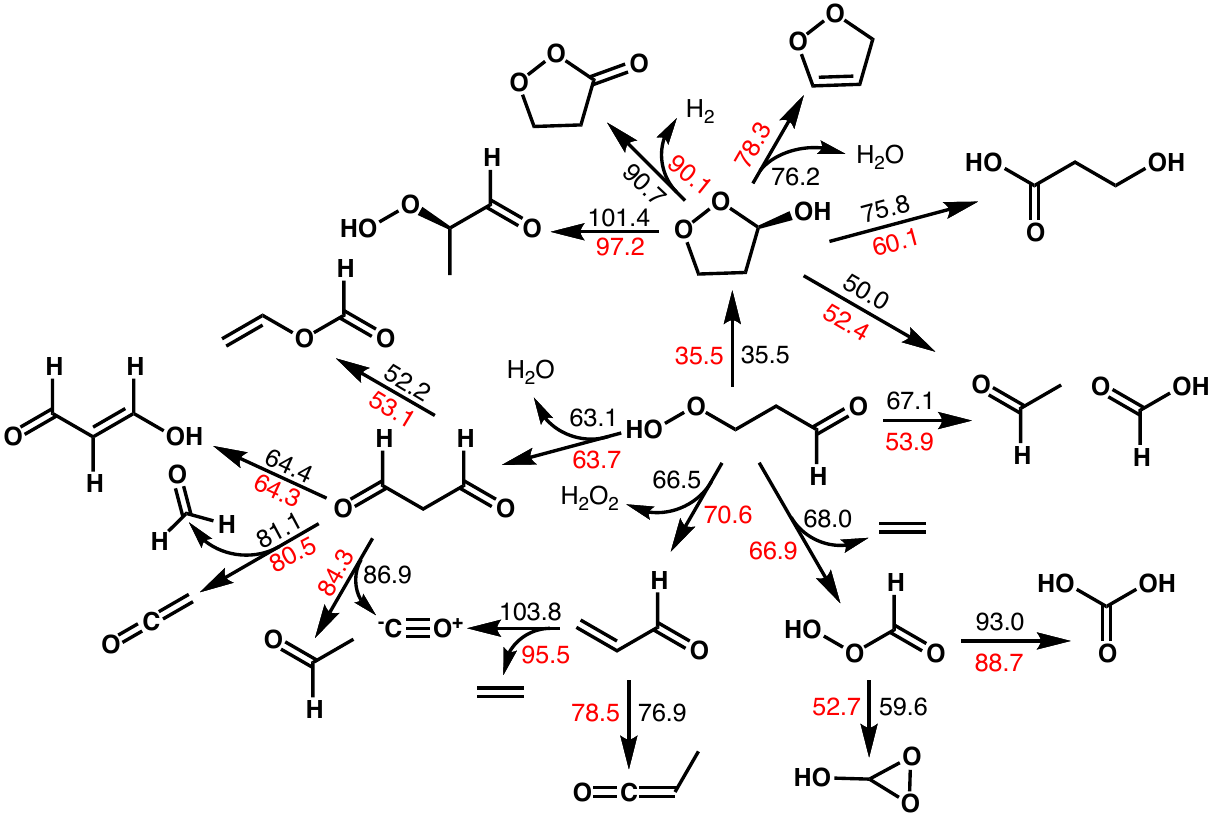}
    % \vspace{-5 pt}
    \caption{\textbf{Reaction Network}}
    \label{Supp:KHPNET}
    % \vspace{-10 pt}
\end{figure*}

% Ablation studies
% \clearpage
\begin{table*}[th]
\centering 
\caption{\textbf{Ablation studies comparing OA-ReactDiff performance on RMSD evaluation with different models}.
Vanilla SE(3) LEFTNet\cite{leftnet} is shown to demonstrate the importance of preserve object-wise symmetry in elementary reaction. EGNN\cite{EGNN} is shown to reflect the importance of vanilla SE(3) model.
}
\resizebox{0.4\textwidth}{!}{
\begin{tabular}{l|cc}\toprule
\multicolumn{1}{c|}{Approach} &\multicolumn{2}{c}{RMSD (Å)} \\\midrule
&mean &median\\\midrule
Object-aware SE(3) LEFTNet&0.183&0.076\\
Vanilla SE(3) LEFTNet&0.638&0.620\\
Object-aware SE(3) EGNN&0.372&0.360\\
\bottomrule
\end{tabular}}
\label{SI:ablation}
\end{table*}

\begin{figure*}[t!]
    % \centering
    \includegraphics[width=1.0\textwidth]{SI/example_multi_molecule_rxn.pdf}
    % \vspace{-5 pt}
    \caption{\textbf{Mutil-molecular elementary reactions sampled from OA-ReactDiff by specifying reactant and product.} Here, the atom mapping and fragment alignment are randomized to demonstrate the capability of OA-ReactDiff not relying on these factors. The generated TS structure only has a RMSD of 0.03 Å compared to the DFT ($\omega$B97x/6-31G(d)) optimized true TS. Atoms are colored as follows: gray for C, blue for N, red for O, and white for H.
    }
    \label{Supp:example_multi_molecule_rxn}
    % \vspace{-10 pt}
\end{figure*}

% \subsection{Samples from unconditional generation}
\begin{figure*}[t!]
    % \centering
    \includegraphics[width=0.9\textwidth]{SI/reaction_samples.png}
    % \vspace{-5 pt}
    \caption{\textbf{Elementary reactions sampled from OA-ReactDiff by only specifying the chemical composition of interest.} Here, we consider a system that contains one C, H, N, and O is chosen. This chemical composition is absent in the Transition1x dataset, and thus is completely new to the trained OA-ReactDiff model. Atoms are colored as follows: gray for C, blue for N, red for O, and white for H.
    }
    \label{Supp:unconditional_samples}
    % \vspace{-10 pt}
\end{figure*}

\begin{figure*}[t!]
    % \centering
    \includegraphics[width=0.7\textwidth]{SI/rmsd_scaling.pdf}
    % \vspace{-5 pt}
    \caption{\textbf{RMSD vs. the number of training data}.
    Mean (top) and median (bottom) RMSD for OA-ReactDiff models trained on different number of training data that are either randomly sampled (blue) or sampled under the constraint that only systems within 15 atoms in size (red) from the original 9000 training reactions.
    }
    \label{Supp:rmsd_scaling}
    % \vspace{-10 pt}
\end{figure*}

\begin{table*}[th]
\centering 
\caption{\textbf{Resource utilization of OA-ReactDiff inference.} Runtime and GPU memory consumption with different batch sizes.
}
\resizebox{0.8\textwidth}{!}{
\begin{tabular}{l|ccccccccc}\toprule
% \multicolumn{1}{c|}{Approach} &\multicolumn{2}{c}{RMSD (Å)} \\\midrule
% &mean &median\\\midrule
batch size&1&2&4&8&16&32&64&128&256\\
walltime (sec)&17.1&18.9&28.0&44.7&87.1&171.8&322.9&582.1&1106.1\\
runtime per sample (sec)&17.1&9.5&7.0&5.6&5.4&5.4&5.1&4.6&4.3\\
GPU memory (GB)&1.1&1.3&1.4&1.6&2.2&3.6&5.7&11.2&21.8\\
\bottomrule
\end{tabular}}
\label{SI:runtime_vs_bs}
\end{table*}

\begin{table*}[th]
\centering 
\caption{\textbf{Performance of OA-ReactDiff.} RMSD at different number of training data and constraints for OA-ReactDiff.
}
\resizebox{0.65\textwidth}{!}{
\begin{tabular}{l|cccc}\toprule
number of sample&1000&5000&5734&9000\\
mean RMSD (Å)&0.453&0.252&0.240&0.183\\
median RMSD (Å)&0.424&0.174&0.180&0.076\\
constraints in training data&--&--&system size < 15 atoms&--\\
\bottomrule
\end{tabular}}
\label{SI:training_data_scaling}
\end{table*}

\begin{figure*}[t!]
    % \centering
    \includegraphics[width=1.0\textwidth]{SI/rmsd_size_box.pdf}
    % \vspace{-5 pt}
    \caption{\textbf{Distributions of RMSD binned by system size.}
    The RMSD is computed between top-1 confidence TS structure generated by OA-ReactDiff and the true TS structure for the 1073 test reactions. A standard box plot with median as the horizontal bar, quartile 1 (Q1) to quartile 3 (Q3) as box edge, and the whiskers correspond to the edges +/- 1.5 times the interquartile range (or, IQR= Q3-Q1) is shown with all RMSDs at that system size displayed on its left hand side.
    }
    \label{Supp:rmsd_size_box}
    % \vspace{-10 pt}
\end{figure*}

% \subsection{Metrics vs. number of runs for OA-ReactDiff}
\begin{figure*}[t!]
    % \centering
    \includegraphics[width=0.7\textwidth]{SI/mae_vs_runs.png.png}
    % \vspace{-5 pt}
    \caption{\textbf{Mean absolute energy difference vs. number of runs for OA-ReactDiff sampling.}. A log-log axis is used to shown the near power law dependence. The results are shown on 1073 test elementary reactions.
    }
    \label{Supp:metric_vs_runs}
    % \vspace{-10 pt}
\end{figure*}

\begin{figure*}[t!]
    % \centering
    \includegraphics[width=0.6\textwidth]{SI/regressor_confidence_ED.pdf}
    % \vspace{-5 pt}
    \caption{\textbf{Performance of using a RMSD regressor as the confidence model}.
    a. Cumulative probability for RMSD between the true TS structures and OA-ReactDiff samples on
    1073 set-aside test reactions. The OA-ReactDiff samples are evaluated under one-shot generation (blue), the top-1 confidence sample via classifier-based recommender (green), and the top-1 confidence sample via RMSD regressor out of 40 generated samples for each reaction (red). A log scale of the RMSD is presented for better visibility of the low-RMSD region. 
    b. 2D density map for the RMSD vs. top-1 RMSD regressor confidence for OA-ReactDiff generated samples. A log-scale color gradient is applied to the color bar to reveal low-density areas, which would otherwise be difficult to distinguish. A histogram of relative probability (prob.) is shown for each axis.
    c. MAE of $|\Delta \mathit{E}_\mathrm{TS}|$ (blue, left y-axis) and the corresponding confidence threshold (orange, right y-axis) as a function of the fraction of data considered in the 1073 TS structures selected via the RMSD regressor.
    }
    \label{Supp:regressor_confidence}
    % \vspace{-10 pt}
\end{figure*}

% \subsection{Highly sensitive example of $\mathrm{C_4 H_6 O_2}$}
\begin{figure*}[t!]
    % \centering
    \includegraphics[width=0.7\textwidth]{SI/C4H6O2.png}
    % \vspace{-5 pt}
    \caption{\textbf{Absolute energy difference vs. RMSD for the ten interpolated structure between true (left) and OA-ReactDiff TS (right) for $\mathrm{C_4 H_6 O_2}$.} The abrupt change in energy difference indicates a change in converged electronic state for self-consistent field calculation.
    }
    \label{Supp:C2H6O2}
    % \vspace{-10 pt}
\end{figure*}

% \subsection{Example of TS with two weakly-interacting fragments}
\begin{figure*}[t!]
    % \centering
    \includegraphics[width=0.7\textwidth]{SI/312_frag.png}
    % \vspace{-5 pt}
    \caption{\textbf{Overlapping OA-ReactDiff and true TS structures of $\mathrm{C_6 H_{10} O}$ separated as two fragments and their corresponding RMSD.} Atoms are colored as follows: C in the true TS structure are in tan and those in the OA-ReactDiff sample are in skyblue; O for red, and H for white.
    }
    \label{Supp:C6H10O}
    % \vspace{-10 pt}
\end{figure*}

% \subsection{Performance on reactions with single vs. multiple reactants and products}
\begin{figure*}[t!]
    % \centering
    \includegraphics[width=0.7\textwidth]{SI/single_vs_multi_products.png}
    % \vspace{-5 pt}
    \caption{\textbf{Box plot for absolute energy difference of OA-ReactDiff + rec. TS structures grouped by single (i.e., n=1) and multi (i.e., n > 1) product cases.}. The median is shown as the horizontal bar, quartile 1 (Q1) to quartile 3 (Q3) as box edge, and the whiskers corresponding to the edges +/- 1.5 times the interquartile range (or, IQR= Q3-Q1). The dashed lines are shown for the mean and standard deviation. The results are shown on 1073 test elementary reactions. 
    }
    \label{Supp:num_prod}
    % \vspace{-10 pt}
\end{figure*}

\begin{table*}[th]
\centering 
\caption{\textbf{Barrier height error of OA-ReactDiff evaluated by different methods}. All energies are reported in the unit of kcal/mol.
}
\resizebox{0.8\textwidth}{!}{
\begin{tabular}{l|ccccccc}\toprule
\multicolumn{1}{c|}{Approach} &\multicolumn{2}{c}{$\omega$B97x}&\multicolumn{2}{c}{B3LYP} &\multicolumn{2}{c}{PBE} &\multicolumn{1}{c}{data fraction}\\\midrule
&mean &median&mean &median&mean &median&\\\midrule
OA-ReactDiff + rec.&4.4&1.6&4.3&1.6&4.9&1.7&1.0\\
OA-ReactDiff + rec. (p>0.5)&3.1&1.4&3.0&1.4&3.7&1.6&0.86\\
\bottomrule
\end{tabular}}
\label{SI:method_dependence}
\end{table*}

% \subsection{Fit comparison of different approaches}
\begin{figure*}[t!]
    % \centering
    \includegraphics[width=0.9\textwidth]{SI/fit_comparison_ED.png}
    % \vspace{-5 pt}
    \caption{\textbf{Absolute energy difference vs. RMSD.} The corresponding linear fit in a log-log plot for OA-ReactDiff + rec. (blue), PSI-based model\cite{ChoiNatComm} (green), and NeuralNEB\cite{NeuralNEB} (orange)}.
    \label{Supp:fit_compare}
    % \vspace{-10 pt}
\end{figure*}
